# Supplementary material for: Sustaining Rabi oscillations by using a phase-tunable image drive
Source: arXiv:2205.14863 ancillary file (2022-05-30)
Supplement: Supplementary file 1 [file s9.pdf]

# Supplemental Material: Sustaining Rabi oscillations by using a phase-tunable image drive

## I. TRANSFORMATION TO THE ROTATING FRAME

This transformation is accomplished by substituting $|\psi(t)\rangle = U|\Psi(t)\rangle$ in the time-dependent Schrödinger equation (TDSE) $i\partial|\psi(t)\rangle/\partial t = H_S|\psi(t)\rangle$ and choosing $U = \exp(i\omega t S^z)$. We have

$$i\frac{\partial}{\partial t}|\Psi(t)\rangle = \left(-iU^\dagger\frac{\partial}{\partial t}U + U^\dagger H_S U\right)|\Psi(t)\rangle \equiv H_{\rm RF}|\Psi(t)\rangle \; . \tag{S1}$$

Using the identity $e^{-i\omega t S^z}S^x e^{+i\omega t S^z} = S^x\cos\omega t + S^y\sin\omega t$ we find

$$\begin{aligned}U^\dagger H_S U = -\omega_0 S^z - \omega_d S^x&\left(\sin\{[2\pi(f_0+\Delta)-\omega]t+\phi\}+\sin\{[2\pi(f_0+\Delta)+\omega]t+\phi\}\right)\\ -\omega_d S^y&\left(\cos\{[2\pi(f_0+\Delta)-\omega]t+\phi\}-\cos\{[2\pi(f_0+\Delta)+\omega]t+\phi\}\right)\\ -\omega_i S^x&\left(\sin\{[2\pi(f_0-\Delta)-\omega]t-\phi\}+\sin\{[2\pi(f_0-\Delta)+\omega]t-\phi\}\right)\\ -\omega_i S^y&\left(\cos\{[2\pi(f_0-\Delta)-\omega]t-\phi\}-\cos\{[2\pi(f_0-\Delta)+\omega]t-\phi\}\right) \; .\end{aligned} \tag{S2}$$

Using the standard argument that we may omit terms that oscillate with the (very large) frequency $2\omega_0$, the Hamiltonian in the rotating frame reads

$$\begin{aligned}H_{\rm S,RF}(t) &\equiv -iU^\dagger\frac{\partial}{\partial t}U + U^\dagger H_S U\\ &= 2\pi\left\{\Delta S^z - h_d\left(S^x\sin\phi + S^y\cos\phi\right) + h_i\left[S^x\sin(4\pi t\Delta+\phi) - S^y\cos(4\pi t\Delta+\phi)\right]\right\} = -\mathbf{B}(t)\cdot\mathbf{S} \; ,\end{aligned} \tag{S3}$$

where

$$\mathbf{B}(t) = 2\pi\begin{pmatrix} h_d\sin\phi - h_i\sin(4\pi t\Delta+\phi)\\ h_d\cos\phi + h_i\cos(4\pi t\Delta+\phi)\\ \Delta\end{pmatrix} \; . \tag{S4}$$

Obviously, we can perform another transformation to a new rotating frame, eliminating the motion associated with the time-independent terms in Eq. (S3). First, we write Eq. (S3) in the more condensed form

$$H_{\rm S,RF}(t) = 2\pi\left[F_{\rm R}\,\mathbf{u}\cdot\mathbf{S} + h_i\mathbf{v}(t)\cdot\mathbf{S}\right] \; , \tag{S5}$$

where $\mathbf{u} = F_{\rm R}^{-1}\left(-h_d\sin\phi, -h_d\cos\phi, \Delta\right)^{\rm T}$ and $\mathbf{v}(t) = (\sin(4\pi\Delta t+\phi), -\cos(4\pi\Delta t+\phi), 0)^{\rm T}$ are unit vectors and $F_{\rm R}^2 = \Delta^2 + h_d^2$. The time-independent term in Eq. (S5) can be eliminated from the TDSE through the unitary transformation $V = \exp(-2\pi i t F_{\rm R}\,\mathbf{u}\cdot\mathbf{S})$. Substituting $|\Psi(t)\rangle = V|\Phi(t)\rangle$ in the TDSE, we find

$$i\frac{\partial}{\partial t}|\Phi(t)\rangle = 2\pi h_i\, e^{2\pi i t F_{\rm R}\,\mathbf{u}\cdot\mathbf{S}}\,\mathbf{v}(t)\cdot\mathbf{S}\, e^{-2\pi i t F_{\rm R}\,\mathbf{u}\cdot\mathbf{S}}|\Phi(t)\rangle = H_{\rm S,RF,RF}(t)|\Phi(t)\rangle \; . \tag{S6}$$

Making use of the identity

$$e^{i\varphi\mathbf{u}\cdot\mathbf{S}}\,\mathbf{v}(t)\cdot\mathbf{S}\,e^{-i\varphi\mathbf{u}\cdot\mathbf{S}} = \left[\mathbf{v}(t)\,\cos\varphi - \mathbf{u}\times\mathbf{v}(t)\,\sin\varphi + \mathbf{u}\cdot\mathbf{v}(t)\,\mathbf{u}\,(1-\cos\varphi)\right]\cdot\mathbf{S} \; . \tag{S7}$$

we find

$$\begin{aligned}H_{\rm S,RF,RF}(t) = 2\pi h_i&\left[-\frac{\Delta}{F_{\rm R}}\cos(4\pi t\Delta+\phi)\sin(2\pi t F_{\rm R}) + \cos(2\pi t F_{\rm R})\sin(4\pi t\Delta+\phi) - \frac{2h_d^2}{F_{\rm R}^2}\sin\phi\cos(4\pi t\Delta+2\phi)\sin^2(\pi t F_{\rm R})\right]S^x\\ -2\pi h_i&\left[\frac{\Delta}{F_{\rm R}}\sin(4\pi t\Delta+\phi)\sin(2\pi t F_{\rm R}) + \cos(2\pi t F_{\rm R})\cos(4\pi t\Delta+\phi) + \frac{2h_d^2}{F_{\rm R}^2}\cos\phi\cos(4\pi t\Delta+2\phi)\sin^2(\pi t F_{\rm R})\right]S^y\\ +4\pi h_i\sin(\pi t F_{\rm R})&\left[\frac{\Delta h_d}{F_{\rm R}^2}\cos(4\pi t\Delta+2\phi)\sin(\pi t F_{\rm R}) - \frac{h_d}{F_{\rm R}}\cos(\pi t F_{\rm R})\sin(4\pi t\Delta+2\phi)\right]S^z \; .\end{aligned} \tag{S8}$$

Part of the Hamiltonian Eq. (S8) becomes time independent if $F_\mathrm{R} = 2\Delta$, in which case we have

$$\begin{aligned} H_{\mathrm{S,RF,RF}}(t) = &\frac{3\pi h_i}{2}\left[\sin\phi\, S^x - \cos\phi\, S^y\right] \\ &+\frac{\pi h_i}{\Delta^2}\left[\frac{1}{2}\sin(8\pi t\Delta+\phi) - h_d^2 \sin\phi\cos(4\pi t\Delta+2\phi)\sin^2(2\pi t\Delta)\right] S^x \\ &-\frac{\pi h_i}{\Delta^2}\left[\frac{1}{2}\cos(8\pi t\Delta+\phi) + h_d^2 \cos\phi\cos(4\pi t\Delta+2\phi)\sin^2(2\pi t\Delta)\right] S^y \\ &-\frac{2\pi h_i h_d}{4\Delta}\sin(2\pi t\Delta)\left[3\sin(4\pi t\Delta+2\phi)+\sin(6\pi t\Delta+2\phi)\right] S^z\,. \end{aligned} \tag{S9}$$

The first term induces a "second" Rabi oscillation with frequency $F_R^{(2)} = 3h_i/4$. In the case of the first transformation to the rotating frame, the fact that $f_0 \gg \Delta$, $f_0 \gg h_d \gg h_i$ can be used to argue that we may drop the fast-oscillating, time dependent terms. However, this line of reasoning cannot be use to argue away the time-dependent terms in Eq. (S9), not even at the second resonance condition $F_\mathrm{R} = 2\Delta$ because the time scales involved are not that different. Repeating the calculation that led to Eq. (S9) for $F_\mathrm{R} = 3\Delta, 4\Delta$, that is for the condition of the second and third Floquet resonance, respectively, does not yield an Hamiltonian that contains time-independent terms. Thus, in these two cases, there is no "second" Rabi oscillation. Note that the results of this section are valid for any value of the spin $S$.

It is instructive to look at the time evolution of the magnetization if we only keep the time-independent term in Eq. (S9). In this approximations, the spin will perform a "second" rotation about the vector $(\sin\phi, -\cos\phi, 0)^\mathbf{T}$ with a frequency $F_R^{(2)} = 3h_i/4$, that is with a frequency determined by the amplitude of the image drive. For $h_i = 0.12h_d = 1.8\,\mathrm{MHz}$ [S1], $F_R^{(2)} = 1.35\,\mathrm{MHz}$, corresponding to a second Rabi oscillation period $P_R^{(2)} = 0.74\,\mu\mathrm{s}$.

Taking $\phi = 0^\circ$ for simplicity we have

$$|\psi(t)\rangle = UV|\Phi(t)\rangle \approx e^{i\omega t S^z} e^{-2\pi i t(\Delta S^z - h_d S^y)} e^{3i\pi h_i t S^y/2}|\Phi(t=0)\rangle\,, \tag{S10}$$

and $|\Phi(t=0)\rangle = \psi(t=0)\rangle$. Restricting ourselves to $S = 1/2$ and assuming that at $t = 0$, the spin is up ($|\Phi(t=0)\rangle = |\uparrow\rangle$), we find

$$\begin{aligned} \langle S^z(t)\rangle \approx &\langle\uparrow| e^{-3i\pi h_i t S^y/2} e^{+2\pi i t(\Delta S^z - h_d S^y)} e^{-i\omega t S^z} S^z e^{i\omega t S^z} e^{-2\pi i t(\Delta S^z - h_d S^y)} e^{3i\pi h_i t S^y/2}|\uparrow\rangle = \\ &\frac{\Delta^2\cos\left(\frac{3}{2}\pi t h_i\right) + h_d^2\cos\left(\frac{3}{2}\pi t h_i\right)\cos\left(2\pi t\sqrt{h_d^2+\Delta^2}\right) - h_d\sqrt{h_d^2+\Delta^2}\sin\left(\frac{3}{2}\pi t h_i\right)\sin\left(2\pi t\sqrt{h_d^2+\Delta^2}\right)}{h_d^2+\Delta^2}\,. \end{aligned} \tag{S11}$$

If $h_i = 0$, Eq. (S11) reduces to

$$\langle\uparrow| e^{+2\pi i t(\Delta S^z - h_d S^y)} S^z e^{-i\omega t S^z} e^{i\omega t S^z} e^{-2\pi i t(\Delta S^z - h_d S^y)}|\uparrow\rangle = \frac{\Delta^2 + h_d^2\cos\left(2\pi t\sqrt{h_d^2+\Delta^2}\right)}{h_d^2+\Delta^2}\,. \tag{S12}$$

If $h_i = 0$, it follows from Eq. (S12) that the magnetization performs Rabi oscillations with an offset of $\Delta^2/(h_d^2+\Delta^2)$. However, if the image drive is present ($h_i \neq 0$), Eq. (S11) shows that the effect of the "second" Rabi oscillation is to reduce this offset to zero.

In the non-resonant case, $F_\mathrm{R} \not\approx 2\Delta$, the Hamiltonian Eq. (S8) determines the motion of the spin in the double-rotating frame. Clearly, with all the time-dependent terms present in Eq. (S8), we cannot expect the motion of the spin to be "simple". Moreover, in the non-resonant case, the transformation to the second rotating frame does not simplify matters relative to Eq. (3). In conclusion: even in the absence of dissipation and decoherence, the presence of the image drive leads to an equation of motion for the spin which, except in the resonant case $F_\mathrm{R} = 2\Delta$, seems very difficult to analyze analytically.

## II. SCHRÖDINGER DYNAMICS OF THE SINGLE-SPIN SYSTEM

To appreciate the complexity of the spin dynamics generated by the time-dependent Hamiltonian Eq. (3), we first consider the case $h_d = 0$ and $h_i \neq 0$ (not realizable experimentally). Then the term in Eq. (3) proportional to $h_i$ can be replaced by a time-independent field proportional to $h_i$ by transforming to a second rotating frame (see section I). This transformation is exact and yields a time-independent Hamiltonian which induces the usual Rabi oscillations of the spin. These oscillations do not depend on value of the phase $\phi$. The initial torque (on the spin aligned along the $z$-axis) is determined by $h_i$.

In contrast, if $h_d \neq 0$, the initial torque on the spin is determined by the second term in Eq. (3) and can, depending on $\phi$, be along any direction in the $x$–$y$ plane. In other words, the motion of the spin generated by the time-dependent Hamiltonian Eq. (3) can, depending on $h_i$ and $\phi$, be quite complicated.

If $h_i = 0$, $\mathbf{B}(t)$ (see Eq. (S4)) is constant in time. It then follows immediately that the spin $\mathbf{S}$ will perform Rabi oscillations with a frequency $F_{\mathrm{R}}^2 = \Delta^2 + h_d^2$. If $\Delta = 0$, the motion is the usual Rabi oscillation about the vector in the direction $(h_d \sin\phi, h_d \cos\phi, 0)^{\mathbf{T}}$. The time average of $\langle S^z(t)\rangle$ is zero. If $\Delta \neq 0$, the spin performs rotations about the vector $(h_d \sin\phi, h_d \cos\phi, \Delta)^{\mathbf{T}}$. The time average of $\langle S^z(t)\rangle = \Delta(\Delta^2 + h_d^2)^{-1/2} \neq 0$.

If $h_i \neq 0$, the spin dynamics is more complicated and can, in general, only be studied numerically. A graphical representation of the spin motion on the Bloch sphere can be obtained using QuTip [S2] for the Hamiltonian parameters of Fig. 2. It is notable how at the Floquet resonance (middle plots) the spin explores the full sphere although the motion is somewhat more complex at $\phi = 45°$ (bottom row) then at $\phi = 0°$ (top row).

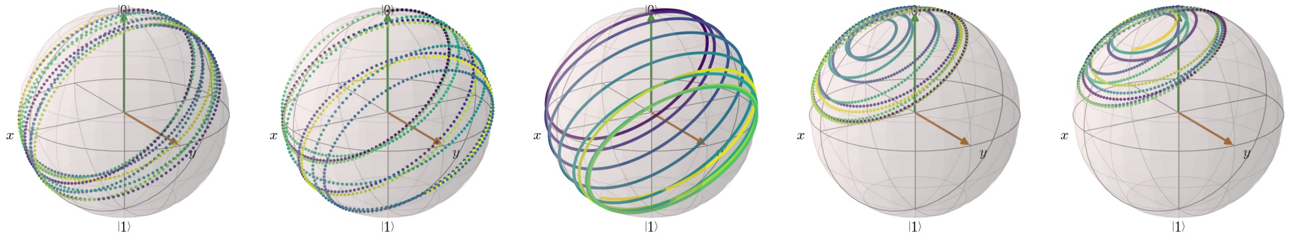


FIG. S1. (color online) Bloch sphere representation of the motion of the spin for the cases shown in Fig. 2(a-e). The brightness of the curve representing the trajectory changes from dark to light as time proceeds.

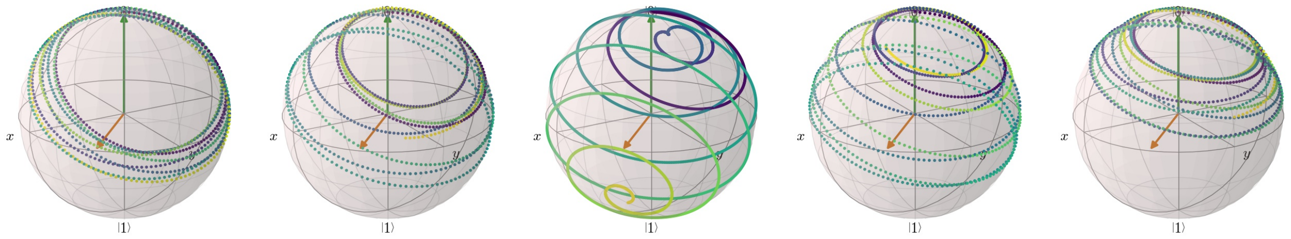


FIG. S2. (color online) Bloch sphere representation of the motion of the spin for the cases shown in Fig. 2(h-j). The brightness of the curve representing the trajectory changes from dark to light as time proceeds.

## III. FLOQUET THEORY

The Hamiltonian Eq. (3) is periodic in time with a frequency $f = 2\Delta$. Therefore, we can resort to Floquet theory to analyze some of its properties. Substituting

$$|\psi(t)\rangle = e^{-2\pi i\kappa t} \sum_{n=-\infty}^{+\infty} e^{-2\pi i f t n} |\psi_n(t)\rangle \,, \tag{S13}$$

in the TDSE

$$i\frac{\partial}{\partial t}|\psi(t)\rangle = H_{\mathrm{S,RF}}(t)|\Psi(t)\rangle \,, \tag{S14}$$

we obtain

$$2\pi\kappa e^{-2\pi i\kappa t} \sum_{n=-\infty}^{+\infty} e^{-2\pi i f t n}|\psi_n(t)\rangle + e^{-2\pi i\kappa t} \sum_{n=-\infty}^{+\infty} (2\pi f n) e^{-2\pi i f t n}|\psi_n(t)\rangle = e^{-2\pi i\kappa t} \sum_{n=-\infty}^{+\infty} e^{-2\pi i f t n} H_{\mathrm{S,RF}}(t)|\psi_n(t)\rangle \,. \tag{S15}$$

Multiply both sides of Eq. (S15) by $e^{+2\pi i\kappa t}$ and $e^{2\pi i f t m}$, integrate over the time interval $[0, f^{-1}]$ and use $f\int_0^{f^{-1}} \exp[2\pi i f t(m-n)] = \delta_{m,n}$, to find

$$\kappa|\psi_m(t)\rangle + fm|\psi_m(t)\rangle = \sum_{n=-\infty}^{+\infty} H_{m-n}|\psi_n(t)\rangle \,, \tag{S16}$$

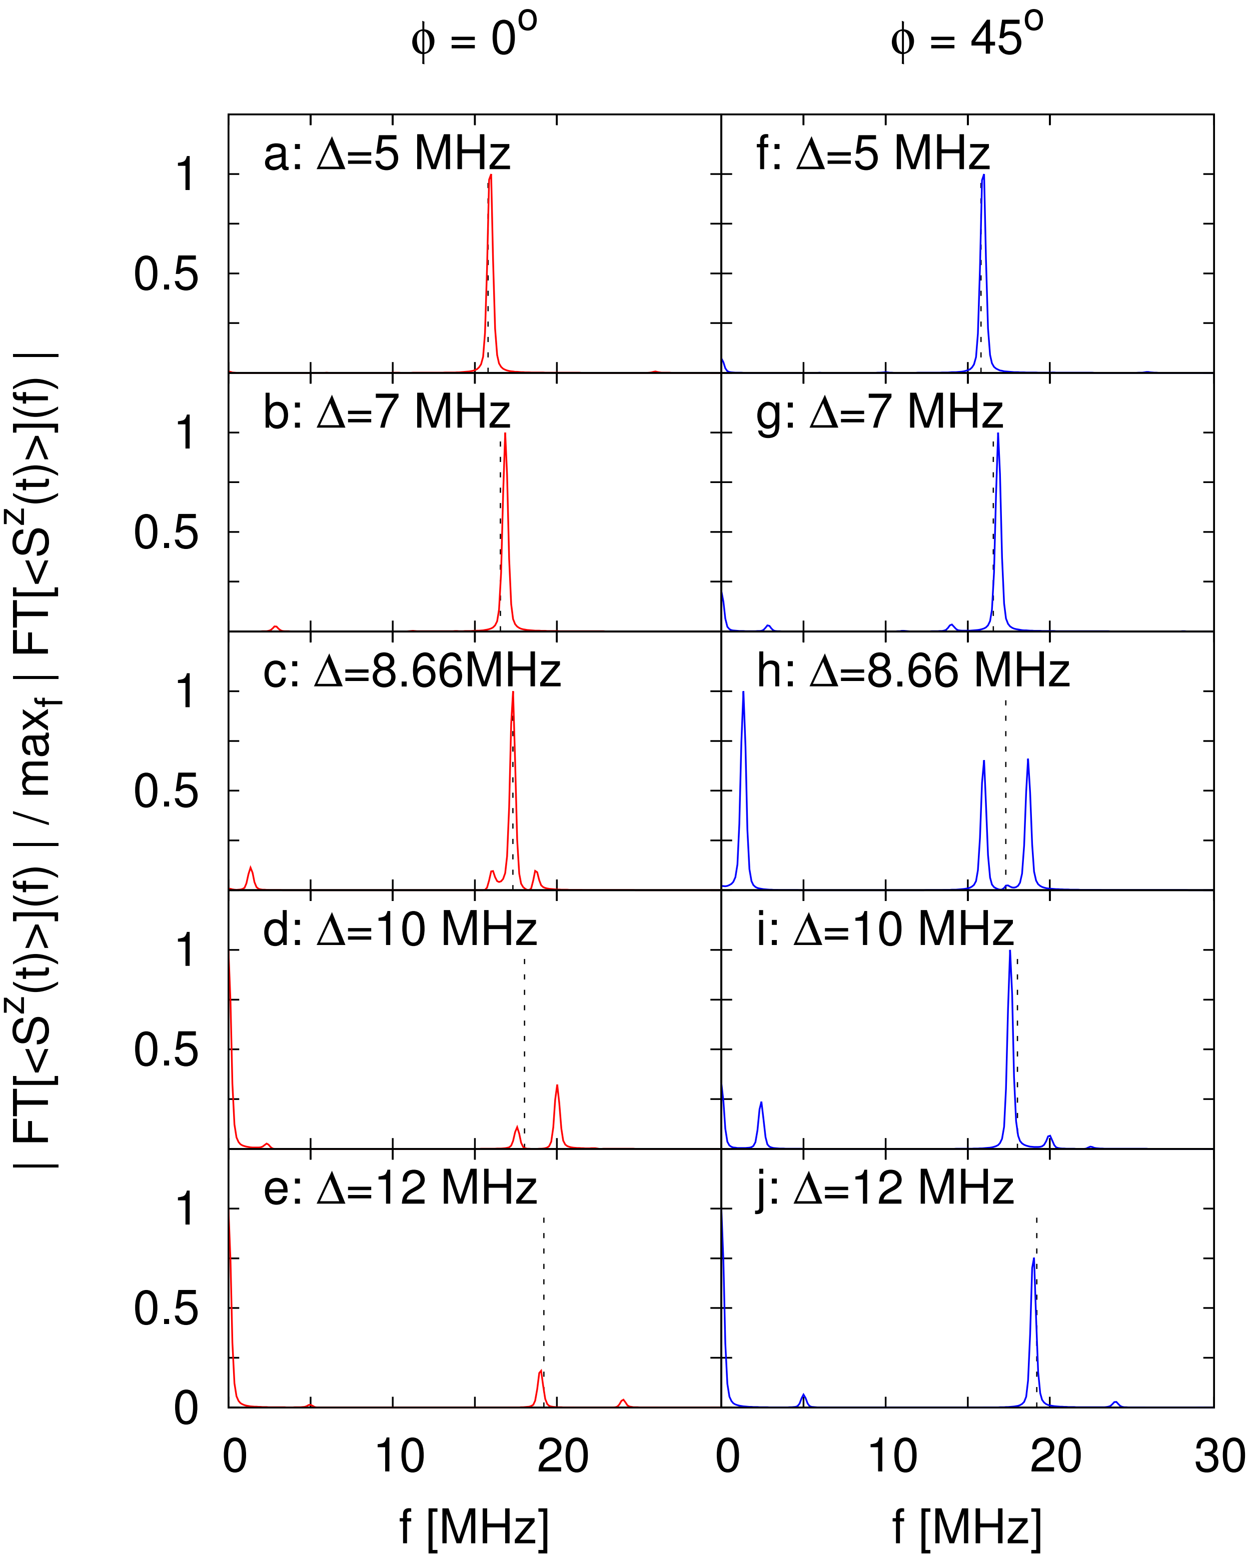


FIG. S3. (color online) Normalized Fourier transforms of the data shown in Fig. 2, that is of the simulation results obtained by solving the TDSE for the Hamiltonian Eq. (3), describing a single spin subject to the time-dependent magnetic field $\mathbf{B}(t) = 2\pi(h_d \sin\phi - h_i \sin(4\pi t\Delta + \phi), h_d \cos\phi + h_i \cos(4\pi t\Delta + \phi), \Delta)^{\mathrm{T}}$, with the amplitudes $h_d = 15\,\mathrm{MHz}$ and $h_i = 0.12 h_d = 1.8\,\mathrm{MHz}$.

where

$$H_{m-n} = \frac{f}{2\pi}\int_0^{f^{-1}} e^{2\pi i f t(m-n)} H_{\mathrm{S,RF}}(t)\,dt = \begin{cases} [\Delta S^z - h_d\,(S^x \sin\phi + S^y\cos\phi)] & , \quad n=m \\ h_i e^{i(\phi-\pi/2)}(S^x + iS^y)/2 & , \quad m-n=+1 \\ h_i e^{-i(\phi-\pi/2)}(S^x - iS^y)/2 & , \quad m-n=-1 \\ 0 & , \quad |n-m|>1 \end{cases} . \tag{S17}$$

Using Eq. (S17), Eq. (S16) reduces to

$$\kappa|\psi_m(t)\rangle = (H_0 - mf\mathbb{1})|\psi_m(t)\rangle + H_{+1}|\psi_{m-1}(t)\rangle + H_{-1}|\psi_{m+1}(t)\rangle \quad , \quad m=-\infty,\dots,+\infty\,. \tag{S18}$$

For simplicity, we restrict ourselves to spin $S=1/2$. Then $|\psi_m(t)\rangle$ is a two-component spinor $|\psi_m(t)\rangle = \left(|\psi_{m,\uparrow}(t)\rangle, |\psi_{m,\downarrow}(t)\rangle\right)^{\mathrm{T}}$ and the matrices that appear in Eq. (S18) read

$$H_0(m) = H_0 - mf\mathbb{1} = \frac{1}{2}\begin{pmatrix} \Delta - 4\Delta m & ih_d e^{-i\phi} \\ -ih_d e^{i\phi} & -\Delta - 4\Delta m \end{pmatrix} , \; H_{+1} = \frac{h_i}{2}e^{i(\phi-\pi/2)}\begin{pmatrix} 0 & 1 \\ 0 & 0 \end{pmatrix} , \; H_{-1} = \frac{h_i}{2}e^{-i(\phi-\pi/2)}\begin{pmatrix} 0 & 0 \\ 1 & 0 \end{pmatrix} . \tag{S19}$$

The eigenvalues of $H_0(m)$ are $\mu_{\pm,m} = -2m\Delta \pm F_R/2$ where $F_R = (\Delta^2 + h_d^2)^{1/2}$ is the Rabi frequency in the absence of the image drive ($h_i = 0$). In the perturbation regime $|h_i| \ll h_d$, the condition for a (Floquet) resonance is $\mu_{-,m} - \mu_{+,m+k} = -2m\Delta - F_R/2 - (-2(m+k)\Delta + F_R/2) = 2k\Delta - F_R = 0$ or $2k\Delta = F_R$, yielding

$$\Delta = \frac{h_d}{\sqrt{4k^2-1}} \quad , \quad k=1,2,\dots\,. \tag{S20}$$

Keeping only the $m=-1,0,1$ contributions in Eq. (S18), we take $(|\psi_{-1}(t)\rangle, |\psi_0(t)\rangle, |\psi_{+1}(t)\rangle)^{\mathrm{T}}$ as the basis for the 6-dimensional Hilbert space. We find the quasi-energies $\kappa$ by diagonalizing the $6\times 6$ matrix

$$A = \begin{pmatrix} H_0(-1) & H_{-1} & 0 \\ H_{+1} & H_0(0) & H_{-1} \\ 0 & H_{+1} & H_0(+1) \end{pmatrix} = \frac{1}{2}\begin{pmatrix} 5\Delta & ih_d e^{-i\phi} & 0 & 0 & 0 & 0 \\ -ih_d e^{i\phi} & 3\Delta & ih_i e^{-i\phi} & 0 & 0 & 0 \\ 0 & -ih_i e^{i\phi} & \Delta & ih_d e^{-i\phi} & 0 & 0 \\ 0 & 0 & -ih_d e^{i\phi} & -\Delta & ih_i e^{-i\phi} & 0 \\ 0 & 0 & 0 & -ih_i e^{i\phi} & -3\Delta & ih_d e^{-i\phi} \\ 0 & 0 & 0 & 0 & -ih_d e^{i\phi} & -5\Delta \end{pmatrix} . \tag{S21}$$

Writing $\det(A-\kappa\mathbb{1}) = 0$ in polynomial form, it follows that the quasi-energies do not depend on $\phi$.

For reference, in Table S1, we present the six smallest (in absolute value) quasi-energies obtained by numerical diagonalization of the $402\times 402$ matrix resulting from truncation to the subspace spanned by the two-component spinors $\{\psi_{-100},\dots,\psi_{-1},\psi_0,\psi_1,\dots,\psi_{100}\}$. Projection onto the subspace defined by the five two-component spinors $\{\psi_{-2},\psi_{-1},\psi_0,\psi_1,\psi_2\}$ seems to be enough for finding the quasi-energies $\kappa$ to four-digit precision. The positions of the peaks in Fig. S3 can, approximately, be related to the sum and differences of the quasi-energies presented in Table S1. Also for reference, in Fig. S4 we show the four levels with the smallest absolute energies, obtained by numerical diagonalization of Eq. (S21), as function of $h_d/\Delta$ and for three different values $h_i/\Delta = 0, 0.2, 0.5$. A qualitative description of the coherence protection mechanisms emerges from the shape of the quasi-energy levels. At the Floquet resonance, the $h_i$ field has the role of opening up a dynamical sweet spot insensitive to noise in $h_d$ and $\Delta$ in first order since the levels are flat. However, it is important to note that our work doesn't stop at such qualitative interpretation. Our numerical simulations discover the microscopic, physical mechanisms developing inside the bath (resonant or non-resonant to the drive).

Some (but not necessarily all) differences of pairs of eigenvalues of $A$ correspond to the frequencies at which the Fourier transform of the magnetization displays a maximum. Of course, this correspondence is only approximate because $A$ does not

TABLE S1. (color online) The Rabi frequency and the six smallest (in absolute value) quasi-energies obtained by solving the Floquet problem Eq. (S18) for the subspace spanned by $\{\psi_{-100},\dots,\psi_{-1},\psi_0,\psi_1,\dots,\psi_{100}\}$ for different values of the offset $\Delta$, $h_d = 15\,\mathrm{MHz}$ and $h_i = 1.8\,\mathrm{MHz}$.

| $\Delta$ | $F_{\mathrm{R}}$ | $\kappa_{\pm 1}$ | $\kappa_{\pm 2}$ | $\kappa_{\pm 3}$ |
|---|---|---|---|---|
| 5.00 | 15.8114 | ±2.0324 | ±7.9676 | ±12.0324 |
| 7.00 | 16.5529 | ±5.5712 | ±8.4289 | ±19.5711 |
| 8.66 | 17.3204 | ±7.9866 | ±9.3334 | ±25.3066 |
| 10.0 | 18.0278 | ±8.7925 | ±11.2075 | ±28.7925 |
| 12.0 | 19.2094 | ±9.4965 | ±14.5036 | ±33.4964 |

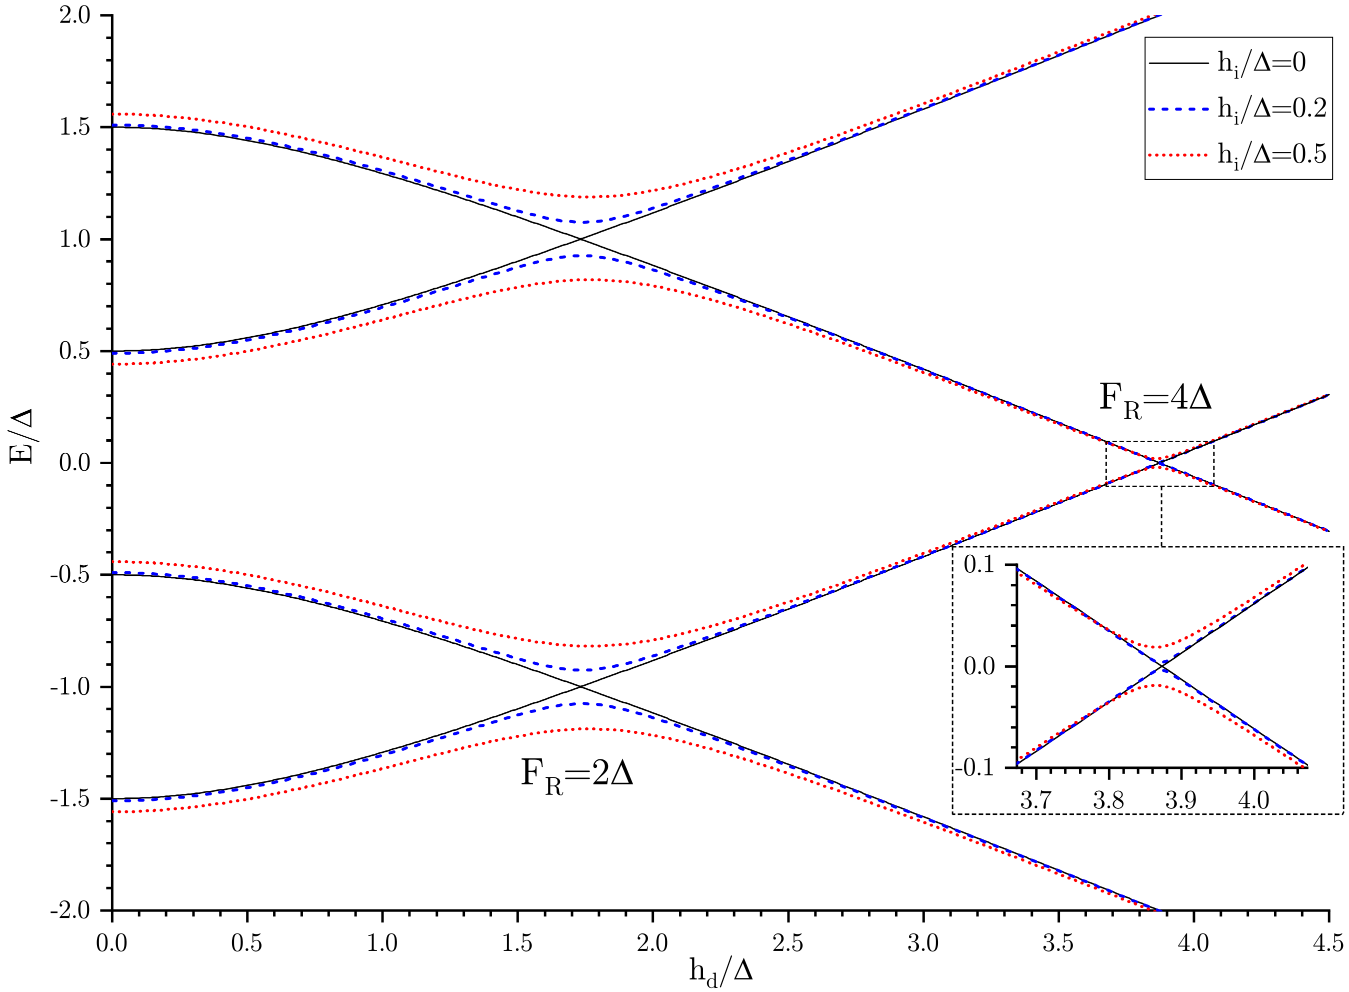


FIG. S4. (color online) Energy level diagram obtained by numerical diagonalization of Eq. (S21). Shown are the four levels with the smallest absolute energies.

account for the $|m| > 1$ contributions. However, this approximation can be quite useful, as we now illustrate by considering the special case of the first Floquet resonance $\Delta = h_d/\sqrt{3}$.

Furthermore, it may also be of interest to note that second-order perturbation theory with respect to $h_i$ yields quite accurate estimates for the eigenvalues of $A$. For $h_d = \sqrt{3}\Delta$ and $h_i = 0$, the six eigenvalues of $A$ are $\pm 3\Delta$, $\pm\Delta$, and $\pm\Delta$. At the first Floquet resonance $h_d/\Delta = \sqrt{3}$, to second order in $h_i$ the eigenvalues of $A$ are $\pm(3\Delta + 7h_i^2/256\Delta)$, $\pm(\Delta - 3h_i/8 + 7h_i^2/512\Delta)$, and $\pm(\Delta + 3h_i/8 + 7h_i^2/512\Delta)$. For our common choice of values of the parameters $h_d = 15\,\mathrm{MHz}$ ($\Delta = 8.66\,\mathrm{MHz}$) and $h_i = 0.12h_d = 1.8\,\mathrm{MHz}$, second-order perturbation theory yields $\pm 7.99012, \pm 9.34012$, and $\pm 25.9902$ (all in MHz), in excellent agreement with the exact diagonalization results mentioned earlier. Also of interest in to note that up to second-order in $h_i^2$, $|\kappa_{\pm 2} - \kappa_{\pm 1}| = 3h_i/4 = F_R^{(2)}$.

For our common choice of values of the parameters $h_d = 15\,\mathrm{MHz}$ ($\Delta = 8.66\,\mathrm{MHz}$) and $h_i = 0.12h_d = 1.8\,\mathrm{MHz}$, exact (numerical) diagonalization of $A$ yields $\pm 25.9904, \pm 9.33913$, and $\pm 7.99121$ (all in MHz). The Fourier spectrum of the magnetization (see Fig. S3(c,h)) shows the main peak at $17.35 \approx (9.34 + 7.99) = 17.33\,\mathrm{MHz}$ which corresponds to the Rabi frequency $F_R = 2\Delta = 17.33\,\mathrm{MHz}$, and two sidebands located at $18.67 \approx (2 \times 9.34) = 18.68\,\mathrm{MHz}$, and $15.99 \approx (2 \times 7.99) = 15.98\,\mathrm{MHz}$, respectively. Clearly, the eigenvalues of the $6 \times 6$ matrix $A$ predict the location of the peaks in the Fourier spectrum quite accurately.

Except for providing guidance to look for resonances, Floquet theory is not of great practical value for computing the time evolution of the single (general) spin, especially since solving the time-dependent Schrödinger equation (TDSE) or the Bloch/Lindblad master equation for a single (general) spin is very easy. In practice, we use the product-formula approach described in Ref. S3 with a time step of 0.1 ns.

## IV. QUANTUM MASTER EQUATION APPROACH

### A. Lindblad quantum master equation

The behavior of the single-spin system S is completely described by the reduced density matrix

$$\rho_{\rm S}(t) \equiv \mathbf{Tr}_{\rm B}\,\rho(t)\;, \tag{S22}$$

where $\rho(t)$ is the density matrix of the whole system $S+B$ at time $t$, $\mathbf{Tr}_{\rm B}$ denotes the trace over the degrees of freedom of the bath, and $\mathbf{Tr}_{\rm S}\,\rho_{\rm S}(t) = \mathbf{Tr}_{\rm S}\,\rho(t) = 1$. In this appendix, we limit ourselves to the case where the system of interest contains only one spin-1/2. Without loss of generality, the reduced density matrix can then be written as

$$\rho_{\rm S}(t) = \frac{1}{2}\left[\mathbb{1}_1 + \sum_{k=1}^{3}\rho_k(t)\sigma_k\right]\;, \tag{S23}$$

where $\rho_{\rm S}(t)$ is the density matrix of the system S, $\mathbb{1}_1$ is the $2\times 2$ unit matrix, $\boldsymbol{\rho}(t) = (\rho_1(t),\rho_2(t),\rho_3(t))$ is a vector of real numbers, and $\boldsymbol{\sigma} = (\sigma_x,\sigma_y,\sigma_z) = (\sigma_1,\sigma_2,\sigma_3)$ are the Pauli matrices. By construction, $\mathbf{Tr}_{\rm S}\,\rho_{\rm S}(t) = 1$. As $\rho_{\rm S}(t)$ is a nonnegative definite matrix, we have $\sum_{k=1}^{3}\rho_k^2(t) \le 1$. From Eq. (S23) it follow immediately that the expectation values of the spin operators are given by

$$\langle\sigma_k(t)\rangle = \mathbf{Tr}_{\rm S}\,\rho_{\rm S}(t)\sigma_k = \rho_k(t) \quad , \quad k=1,2,3\;, \tag{S24}$$

showing that in the case at hand, knowledge of $\langle\sigma_k(t)\rangle$ for $k=1,2,3$ is equivalent to the knowledge of the reduced density matrix $\rho_{\rm S}(t)$. Therefore, in the following, we do not focus on the reduced density matrix itself but on the physically observables $\langle\sigma_x(t)\rangle = 2\langle S^x(t)\rangle = \rho_x(t)$, $\langle\sigma_y(t)\rangle = 2\langle S^y(t)\rangle = \rho_y(t)$, and $\langle\sigma_z(t)\rangle = 2\langle S^z(t)\rangle = \rho_z(t)$.

The Lindblad equation is the most general Markovian master equation describing the time evolution of a density matrix [S4]. The diagonal form of the Lindblad master equation for the reduced density matrix $\rho_{\rm S}(t)$ reads [S4]

$$\frac{d\rho_{\rm S}(t)}{dt} = -i[H_{\rm S,RF}(t),\rho_{\rm S}(t)] + \frac{1}{2}\sum_{j=1}^{3}\gamma_j\left(2A_j\rho_{\rm S}(t)A_j^\dagger - A_j^\dagger A_j\rho_{\rm S}(t) - \rho_{\rm S}(t)A_j^\dagger A_j\right)\;, \tag{S25}$$

where the parameters $\gamma_1,\gamma_2,\gamma_3 \ge 0$. In general, the operators $A_j$ are linear combinations of the matrices that form a basis for the matrices operating on the Hilbert space of the system [S4]. The Lindblad form Eq. (S25) covers all Markovian quantum master equations of which the solution is guaranteed to be a nonnegative definite matrix for all times $t$ [S4].

For the system S consisting of a single spin-1/2, the operators $A_j$ can be written as

$$A_j = \sum_{k=1}^{3}(a_{jk} + ib_{jk})\sigma_k\;, \tag{S26}$$

where the $a_{jk}$'s and $ib_{jk}$'s are real numbers and are the free parameters of the Lindblad model.

Usually, the Lindblad equation Eq. (S25) is solved for the elements of the density matrix and the expectation values of the spin operators are calculated afterwards. For the system S consisting of a single spin-1/2, it is instructive to start from Eq. (S25) and derive the equation of motion for expectation values of the spin operators directly. This facilitates the comparison with the Bloch equations and also helps to give meaning to the many parameters that enter Eq. (S25).

Multiplying Eq. (S25) by $\sigma_l$ and computing the trace, we obtain the equations of motion of the expectation values of the spin-1/2 components $\boldsymbol{\sigma} = (\rho_1,\rho_2,\rho_3)$ (see Eq. (S23)). We have

$$\frac{d\rho_l(t)}{dt} = (\boldsymbol{\rho}\times\mathbf{B}(\mathbf{t}))_l + \frac{1}{2}\sum_{j=1}^{3}\gamma_j\mathbf{Tr}_{\rm S}\,\sigma_l[A_j,A_j^\dagger] + \frac{1}{4}\sum_{j,k=1}^{3}\gamma_j\left[2\mathbf{Tr}_{\rm S}\,\sigma_lA_j\sigma_kA_j^\dagger - \mathbf{Tr}_{\rm S}\,\sigma_lA_j^\dagger A_j\sigma_k - \mathbf{Tr}_{\rm S}\,\sigma_l\sigma_kA_j^\dagger A_j\right]\rho_k(t)\;. \tag{S27}$$

For any choice of the $A_j$'s given by Eq. (S26), the right hand side of Eq. (S27) can be worked out analytically by using the identities $\sigma_p\sigma_q = \delta_{pq} + i\varepsilon_{pqr}\sigma_r$, $\mathbf{Tr}_{\rm S}\,\sigma_p\sigma_q\sigma_r = 2i\varepsilon_{pqr}$, and $\mathbf{Tr}_{\rm S}\,\sigma_p\sigma_q\sigma_r\sigma_s = 2(\delta_{pq}\delta_{rs} - \delta_{pr}\delta_{qs} + \delta_{ps}\delta_{qr})$. However, for this task, it is much more convenient to use Mathematica®. Introducing the symbols $c_{pq} = 2\sum_{j=1}^{3}\gamma_j(a_{jp}a_{jq} + b_{jp}b_{jq})$, and $d_{pq} = 4\sum_{j=1}^{3}\gamma_j(a_{jp}b_{jq} - b_{jp}a_{jq})$, we find that Eq. (S27) can be written as

$$\frac{d}{dt}\begin{pmatrix}\rho_x(t)\\ \rho_y(t)\\ \rho_z(t)\end{pmatrix} = \Big[\boldsymbol{\Omega}(t) - \mathbf{D}\Big]\begin{pmatrix}\rho_x(t)\\ \rho_y(t)\\ \rho_z(t)\end{pmatrix} + \begin{pmatrix}d_{23}\\ d_{31}\\ d_{12}\end{pmatrix} \quad , \quad \mathbf{D} = \begin{pmatrix}c_{22}+c_{33} & -c_{12} & -c_{13}\\ -c_{12} & c_{11}+c_{33} & -c_{23}\\ -c_{13} & -c_{23} & c_{11}+c_{22}\end{pmatrix}\;. \tag{S28}$$

Note that the $c_{pq}$'s and $d_{pq}$'s cannot be chosen independently and that **D** does not depend on time. Apart from the nondiagonal elements in the dissipation matrix, the structure of Eq. (S28) is the same as that of the Bloch equation.

Reference S1 used the Lindblad equation with $A_1 = A_2 = A_3 = \sigma_- = (\sigma_x - i\sigma_y)/2$ as a theoretical model to describe the experimental data. In this case, we have

$$\frac{d}{dt}\begin{pmatrix}\rho_x(t)\\ \rho_y(t)\\ \rho_z(t)\end{pmatrix} = \left[\begin{pmatrix}0 & B_z(t) & -B_y(t)\\ -B_z(t) & 0 & B_x(t)\\ B_y(t) & -B_x(t) & 0\end{pmatrix} - \frac{1}{2}\begin{pmatrix}\gamma & 0 & 0\\ 0 & \gamma & 0\\ 0 & 0 & 2\gamma\end{pmatrix}\right]\begin{pmatrix}\rho_x(t)\\ \rho_y(t)\\ \rho_z(t)\end{pmatrix} + \begin{pmatrix}0\\ 0\\ -\gamma\end{pmatrix}, \tag{S29}$$

where $\gamma = \gamma_1 + \gamma_2 + \gamma_3$. Clearly, Eq. (S29) is of the Bloch form, with $\gamma = 1/T_z$, $T_{xy} = 2T_z$ and $m_0 = -1$. If we choose $A_1 = A_2 = A_3 = \sigma_+ = (\sigma_x + i\sigma_y)/2$, Eq. (S29) remains the same except that $m_0 = +1$.

In order to have a quantum master equation for the single-spin system describe behavior that is significantly different from what the Bloch equation can describe, it may be necessary to allow for an explicit time dependence of the dissipation matrix **D**.

### B. Lindblad equation: simulations results

Figure S5 shows the effect of including decoherence and dissipation on the Rabi oscillations. The values of $T_2 = 2T_1$ and $m_0$ where chosen such that for $\Delta = 5,$MHz, the decay time of the Rabi oscillations is roughly the same as the one observed experimentally. Figure S5(a) shows that the amplitude of the Rabi oscillations vanish on a time scale of about $1\mu$ s. Qualitatively, Figs. 1(a) and S5(a) are similar.

For $\Delta = 7,$MHz, Fig. S5(b) shows sustained Rabi oscillations with a fairly large amplitude over a long period of time, in conflict with the experimental data shown in Fig. 1(b). Comparing Figs. S5(c-f) with Figs. 1(c-f), it is clear that even qualitatively, the Bloch model does not reproduce the main feature (see section I of the experimental data. This conclusion is further supported by the qualitative disagreement between the results for $\phi = 45^\circ$, shown in Figs. S5(f-j) and Figs. 1(f-j),

Comparing the TDSE data (Fig. 3) with the Bloch/Lindblad data (Figs. S5) it is clear that dependence of the Rabi oscillation amplitude on the detuning $\Delta$ and the phase shift $\phi$, exhibited by model Eq. (11), is qualitatively different from that of the Bloch/Lindblad model.

### C. Lindblad equation: Inhomogeneity of the microwave field

In ESR experiments, the microwave fields in the cavity are unlikely to have the same strengths over the whole sample. This inhomogeneity affects the values of $h_d$ and $h_i$, depending on the location of the spins in the sample. In turn, the variation of $h_d$ and $h_i$ itself leads to a decay of the Rabi oscillations, also in the absence of any other source of decoherence/dissipation [S3].

For the single-spin model (see section IV), which we analyze by means of the Bloch equation, it is straightforward to include variations in $h_d$ and $h_i$ by averaging the solutions of the Bloch equation over different choices of $h_d$ and $h_i$. For simplicity, we assume that $h_{d,n} = r_n h_d$ and $h_{i,n} = r_n h_i$. The subscript $n$ labels the instance. The uniform random number $r_n$ is taken from the interval $[1-\delta, 1+\delta]$. The parameter $\delta$ controls the variation of the microwave fields. In all our simulations, we take $\delta = 0.1$. In practice, we solve the Bloch equations for 1000 $(h_{d,n}, h_{i,n})$ instances on a notebook. In Figs. S6 we present some simulation results.

Comparison of Figs. 1 and S6 leads to the conclusion that within the Bloch/Lindblad model, accounting for the inhomogeneity of the microwave fields does not explain the behavior of the amplitude of the long-time magnetization dynamics as a function of $\Delta$ and $\phi$, observed experimentally (see section I).

## V. TECHNICAL ASPECTS OF THE MANY-BODY TDSE SIMULATIONS

The time evolution of a closed quantum system defined by a time-dependent Hamiltonian $H(t)$ is governed by the TDSE

$$i\frac{\partial}{\partial t}|\Psi(t)\rangle = H(t)|\Psi(t)\rangle. \tag{S30}$$

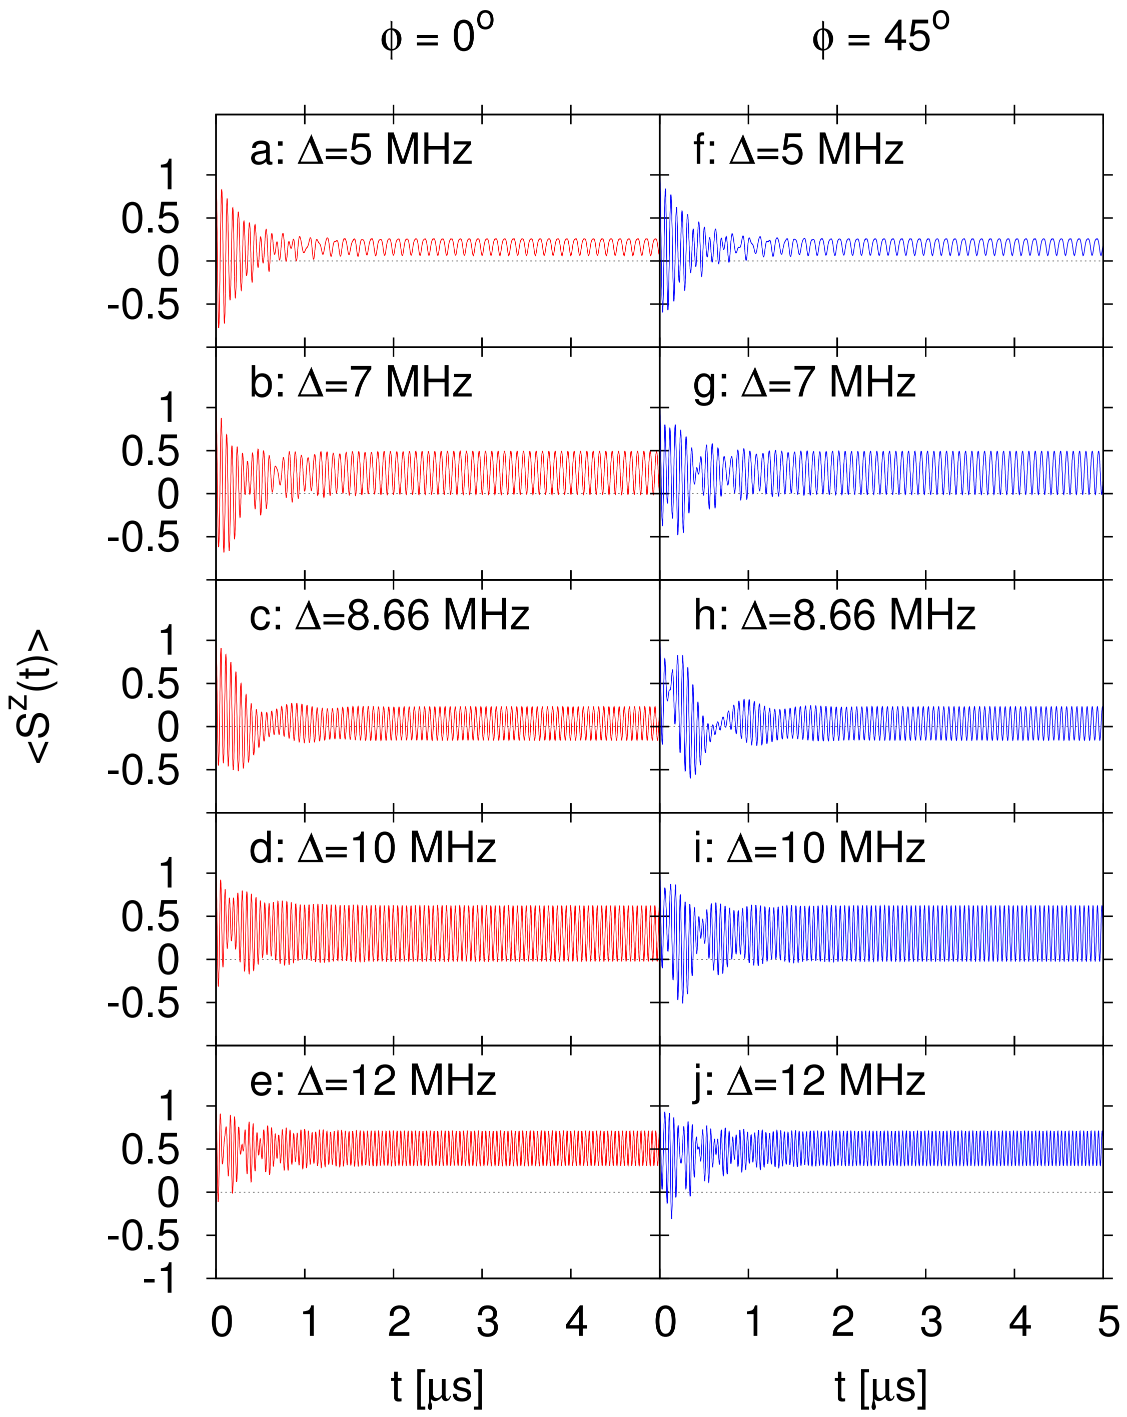


FIG. S5. (color online) Simulation results obtained by solving the Bloch equation for a spin in the time-dependent magnetic field $\mathbf{B}(t) = 2\pi(h_d \sin\phi - h_i \sin(4\pi t\Delta + \phi), h_d \cos\phi + h_i \cos(4\pi t\Delta + \phi), \Delta)^{\mathrm{T}}$ and $1/2T_1 = 1/T_2 = 2\,\mathrm{MHz}$ and $m_0 = 1$, illustrating the effect of the presence on the image drive with strength $h_i$ on the decay of the Rabi oscillations. The values of $h_d = 15\,\mathrm{MHz}$, $h_i = 0.12 h_d = 1.8\,\mathrm{MHz}$, and $\Delta$ are the same as those used to obtain the experimental data shown in Fig. 1.

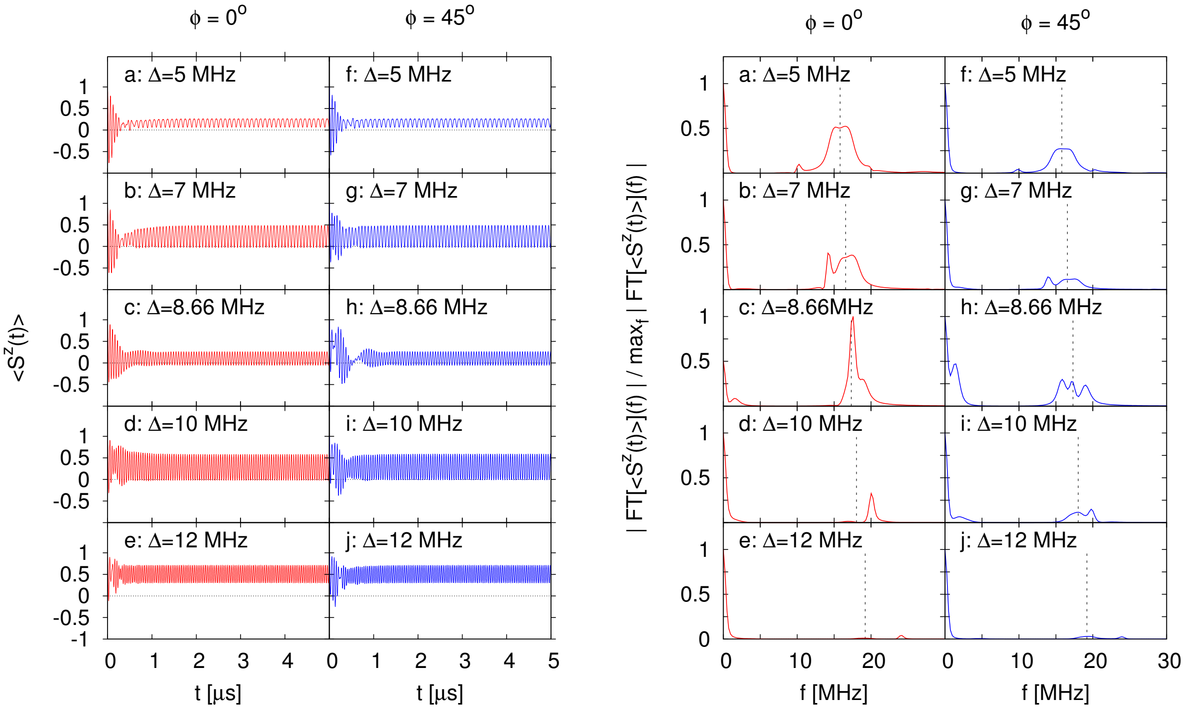


FIG. S6. (color online) Left: Simulation results obtained by averaging 1000 solutions of the Bloch equation for a spin in the time-dependent magnetic field $\mathbf{B}(t) = 2\pi(h_{d,n}\sin\phi - h_{i,n}\sin(4\pi t\Delta+\phi), h_{d,n}\cos\phi + h_{i,n}\cos(4\pi t\Delta+\phi), \Delta)^{\mathrm{T}}$ with $1/2T_1 = 1/T_2 = 2$MHz, $m_0 = 1$, and microwave field inhomogeneity $\delta = 0.1$. illustrating the effect of the inhomogeneity the drive and image drive field on the decay of the Rabi oscillations. Right: Fourier transforms of the data shown in the left panel.

The pure state $|\Psi(t)\rangle$ of the single-spin system + bath at time $t$ can be written as

$$|\Psi(t)\rangle = \sum_{i=\uparrow,\downarrow}\sum_{p=1}^{D_{\mathrm{B}}} c(i,p,t)|i,p\rangle, \tag{S31}$$

where the complete set of the orthonormal states in up–down basis of the system and bath spins is denoted by $\{|i,p\rangle\}$. $D_{\mathrm{S}} = 2$ and $D_{\mathrm{B}} = 2^{N_{\mathrm{B}}}$ are the dimensions of the Hilbert space of the system and bath, respectively. The coefficient $c(i,p,t)$ is the complex-valued amplitude of the state $|i,p\rangle$.

All TDSE simulation results reported in this paper have been obtained by running a massively parallel, quantum spin dynamics simulator (in house software) with a time step of 1 ns for a total of 5000 time steps.

From the knowledge of the $c$'s in Eq. (S31), we can compute any physically relevant property of the system S, the bath B, and the whole system. For instance, the reduced density matrix of the system S reads

$$\rho_{\mathrm{S}}(t) = \begin{pmatrix} |c_\uparrow(t)|^2 & c_\uparrow(t)c_\downarrow^*(t) \\ c_\uparrow^*(t)c_\downarrow(t) & |c_\downarrow(t)|^2 \end{pmatrix} . \tag{S32}$$

where $|c_\uparrow(t)|^2 = \sum_{p=1}^{D_{\mathrm{B}}} |c(\uparrow,p,t)|^2$ etc. From Eq. (S32), we can extract all properties of the system S.

The initial state of the whole system is constructed using the random state technology [S5]. The key feature of random state technology is this: if the dimension $D$ of Hilbert space is large enough, we can obtain an accurate estimate of **Tr** X, the trace of a matrix $X$, by computing $D\langle\Psi|X|\Psi\rangle$ where $|\Psi\rangle$ is a pure state chosen randomly [S5]. This reduces the calculation of averages by a factor $D = 2^{N+1}$, which usually is a large number.

More specifically, to study the Rabi oscillations, the initial state is taken to be a product state of the system S and a thermal pure state of the bath B. As the initial state of the system, we take the state with spin up (along the $z$-axis). The state of the whole system is then given by

$$|\Psi(t=0)\rangle = |\uparrow\rangle_1 \otimes |\Phi(\beta)\rangle \, , \tag{S33}$$

where

$$|\Phi(\beta)\rangle = \frac{e^{-\beta H_{\rm B}/2}|\Phi\rangle}{\langle\Phi|e^{-\beta H_{\rm B}}|\Phi\rangle^{1/2}} \,, \tag{S34}$$

and where $\beta$ denotes the inverse temperature and $|\Phi\rangle$ is a random state of the bath B.

To estimate $\beta\|H_{\rm B}\|/N_{\rm B}$, we assume, for simplicity, that the average energy per bath spin is roughly of the same order of magnitude as the energy of the system spin. To simplify matters even more, we set $H_{\rm B} = h_d N_{\rm B} \mathbb{1}_{N_{\rm B}}$ ($\mathbb{1}_{N_{\rm B}}$ is the $2^{N_{\rm B}} \times 2^{N_{\rm B}}$ unit matrix), and compute $\beta\|H_{\rm B}\|/N_{\rm B}$ in MKS units. Experimentally reasonable values are $T = 40\,$K and $h_d = 15\,$MHz [S1]. Using $k_{\rm B} = 1.38\times 10^{-23}$ (J/K) and $1\,$MHz $= 6.63\times 10^{-28}$ J we have

$$\beta\|H_{\rm B}\| = \frac{1}{k_{\rm B}T}\|H_{\rm B}\| = \frac{15\times 6.63\times 10^{-28}\ {\rm J}}{1.38\times 10^{-23}\ ({\rm J/K})\times 40\ {\rm K}} N_{\rm B} = 1.8\times 10^{-5} N_{\rm B} \,. \tag{S35}$$

This very rough estimate suggests that for the problem at hand, we may think of the bath B being at infinite temperature. Thus, in the simulations of model A, it is sufficient to consider the case $\beta = 0$ only. Note that the arguments that led to the rough estimate Eq. (S35) only involve degrees of freedom that directly interact with the system spin.

From Eq. (S32), it follows immediately that for the initial state Eq. (S33), the reduced density matrix takes the form

$$\rho_{\rm S}(t=0) = \begin{pmatrix} 1 & 0 \\ 0 & 0 \end{pmatrix} \,. \tag{S36}$$

Equation (S36) describes a system in which the spin at $t = 0$ is up, as it should be. As time progresses, the dynamics of the bath and system results in a pure state, a superposition of essentially all possible basis states. If $D_{\rm B}$ is sufficiently large and assuming (for simplicity of the argument) that after a while, the $c(\uparrow, p, t)$'s and $c(\downarrow, p, t)$'s are independent random variables with mean zero, it follows from Eq. (S32) that for all practical purposes, the reduced density matrix can be approximated by

$$\rho_{\rm S}(t\to\infty) = \frac{1}{2}\begin{pmatrix} 1 & 0 \\ 0 & 1 \end{pmatrix} \,. \tag{S37}$$

Then the expectation values of all components of the system spin are zero. Obviously, there is no coherence in the fully mixed state Eq. (S37).

In all sections that report simulation results we abundantly make use of (pseudo)-random numbers to choose the interaction parameters and, as explained below, also to generate the initial state of the spin bath.

To appreciate the reproducibility of the features exhibited by the system spin(s), it is important to keep in mind that every time we perform a simulation, we use different random numbers for the interaction parameters and, if applicable, for the initial state of the bath.

## VI. DEPENDENCE ON THE CHOICE OF RANDOM NUMBERS

In Figs. S7 and S8 we present TDSE simulation data for magnetization and the energy of the bath that show that the dependence on the random initial state and random interaction parameters is negligible.

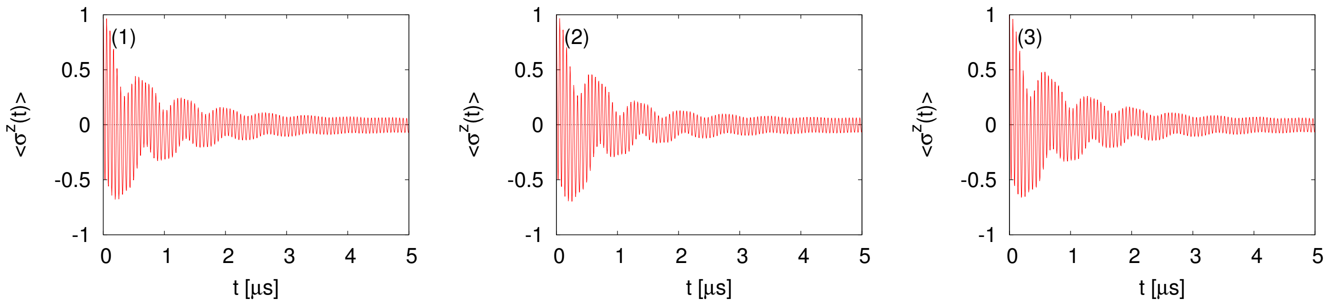


FIG. S7. (color online) Simulation results for the magnetization, as obtained by solving the TDSE Eq. (S30) with Hamiltonian Eq. (11) for a bath with $N_{\rm B} = 28$ spins, spin-bath coupling $\lambda = 6$, $J = 1\,$MHz, $K = 10\,$MHz, $h_d = 15\,$MHz, $h_i = 0.12 h_d = 1.8\,$MHz, and $\Delta = 8.66\,$MHz. All three runs use different random numbers to construct the random initial state and for the interaction parameters. Comparison suggests that the magnetization data are robust with respect to the randomness in the initial state and interaction parameters.

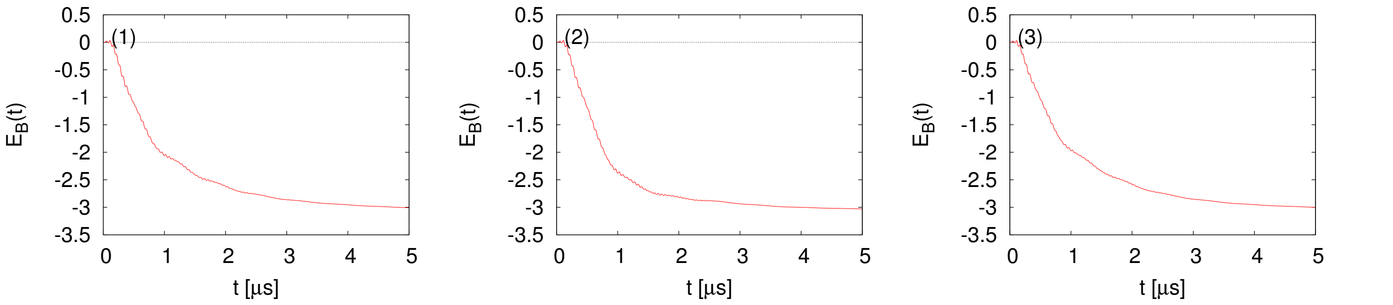

FIG. S8. (color online) Simulation results for the energy of the bath, as obtained by solving the TDSE Eq. (S30) with Hamiltonian Eq. (11) for a bath with $N_\mathrm{B} = 28$ spins, spin-bath coupling $\lambda = 6$, $J = 1\,\mathrm{MHz}$, $K = 10\,\mathrm{MHz}$, $h_d = 15\,\mathrm{MHz}$, $h_i = 0.12h_d = 1.8\,\mathrm{MHz}$, and $\Delta = 8.66\,\mathrm{MHz}$. All three runs use different random numbers to construct the random initial state and for the interaction parameters. Clearly the data for the bath energy are robust with respect to the randomness in the initial state and interaction parameters.

## VII. DEPENDENCE ON THE BATH SIZE

In Figs. S9 and S10 we present TDSE simulation data for magnetization and system, bath and total energy to show that changing the number of bath spins $N_\mathrm{B} = 14, 28, 32$ has little effect on data.

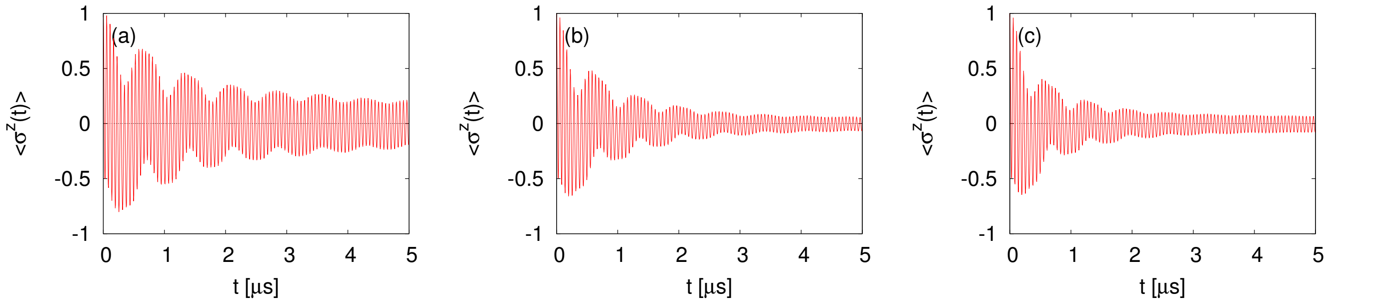

FIG. S9. (color online) Simulation results for the magnetization, as obtained by solving the TDSE Eq. (S30) with Hamiltonian Eq. (11) for a spin-bath coupling $\lambda = 6$, $J = 1\,\mathrm{MHz}$, $K = 10\,\mathrm{MHz}$, $h_d = 15\,\mathrm{MHz}$, $h_i = 0.12h_d = 1.8\,\mathrm{MHz}$, and $\Delta = 8.66\,\mathrm{MHz}$. a: $N_\mathrm{B} = 14$; b: $N_\mathrm{B} = 28$; c: $N_\mathrm{B} = 32$. These data suggest that the main features of the magnetization are fairly robust with respect to the size of the spin bath.

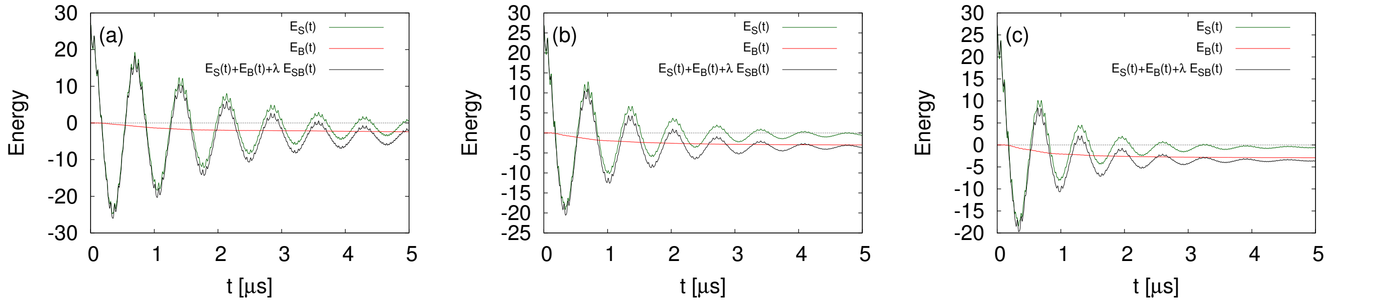

FIG. S10. (color online) Simulation results for the system, bath, and total energy, as obtained by solving the TDSE Eq. (S30) with Hamiltonian Eq. (11) for a spin-bath coupling $\lambda = 6$, $J = 1\,\mathrm{MHz}$, $K = 10\,\mathrm{MHz}$, $h_d = 15\,\mathrm{MHz}$, $h_i = 0.12h_d = 1.8\,\mathrm{MHz}$, and $\Delta = 8.66\,\mathrm{MHz}$. a: $N_\mathrm{B} = 14$; b: $N_\mathrm{B} = 28$; c: $N_\mathrm{B} = 32$. These data suggest that the system, bath, and total energy are fairly robust with respect to the size of the spin bath.

## VIII. ENERGIES OF THE MODELS EQS. (11) AND (17)

For completeness, in Figs. S11 and S12 we present TDSE simulation data of the system spin, the spin bath and the total energy for the same cases as those that yield that data shown in Fig. 3. Note that Fig. S11(c) and Fig. S12(c) also appear in the main text as Fig. 4. In Figs. S13 and S14 we present TDSE simulation data of the total energy of the system per spin $E_\mathrm{S}/N_\mathrm{S} = \langle\Psi(t)|H(t)|\Psi(t)\rangle/N_\mathrm{S}$, for the same sets of model parameters as those that yield that data shown in Fig. 6.

At the Floquet resonance $2\Delta = F_R$ (corresponding to panels (c)), all the total energies perform damped oscillations with the "second" Rabi frequency $F_R^{(2)}$. Away from the Floquet resonance, the behavior of the total energy is atypical, very much depending on $\Delta$, $\phi$ and on whether we consider the model Eq. (11) or Eq. (17.

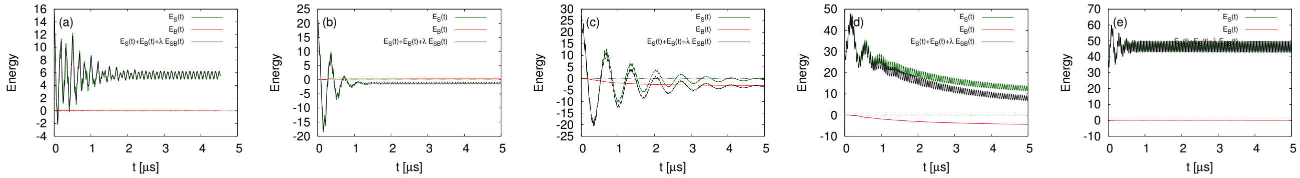


FIG. S11. (color online) Simulation results for the energy of the system, bath and total energy, as obtained by solving the TDSE Eq. (S30) with Hamiltonian Eq. (11) for a bath with $N_\mathrm{B} = 28$ spins, spin-bath coupling $\lambda = 6$. For the values of the model parameters, see Fig. 3.

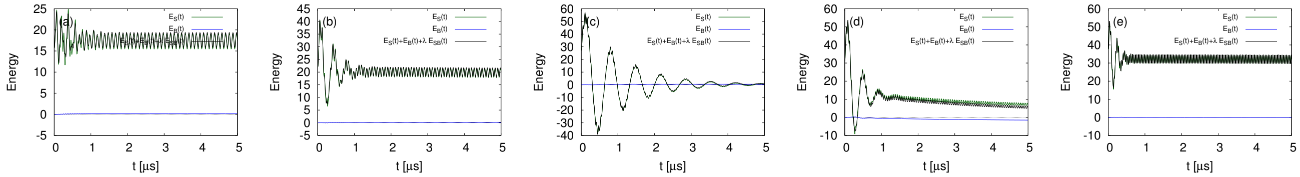


FIG. S12. (color online) Same as Fig. S11 except that $\phi = 45°$.

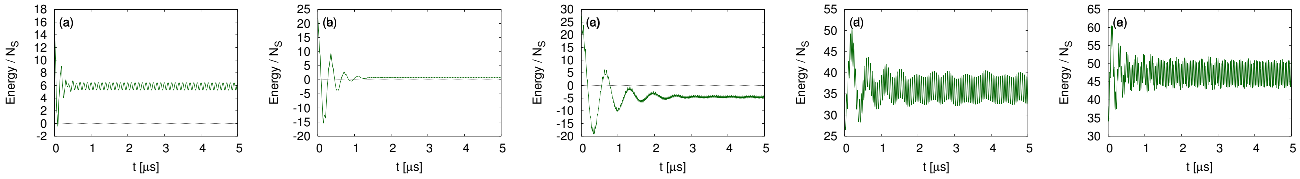


FIG. S13. (color online) Simulation results for the total energy, as obtained by solving the TDSE Eq. (S30) with Hamiltonian Eq. (15) for a system with $N_\mathrm{S} = 28$ spins, spin-bath coupling $\lambda = 5$. For the values of the model parameters, see Fig. 6.

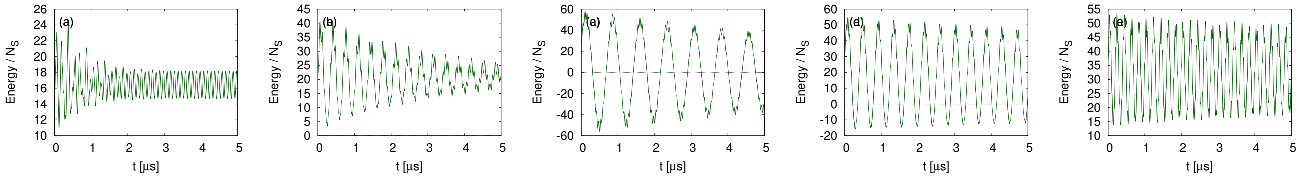


FIG. S14. (color online) Same as Fig. S13 except that $\phi = 45°$.

## IX. SPIN-SPIN CORRELATIONS IN MODEL EQS. (17)

Here we present the time dependence of the spin-spin correlations in the case of a system of interacting spins resonant to the microwave field. In panel (a) of Fig. S15 the image drive is not fulfilling the Floquet resonance and any sign of correlation quickly vanishes. When the Floquet condition is met, see panel (b), one observes long standing oscillations although the Floquet

mode for $\phi = 45^\circ$ has the effect of beatings and a decrease of the overal amplitude. In both panels, the case $h_i = 0$ represent a regular Rabi oscillation of the main spin, without our protocol in place. This leads to a quick dephasing, without any trace of internal correlations in the bath.

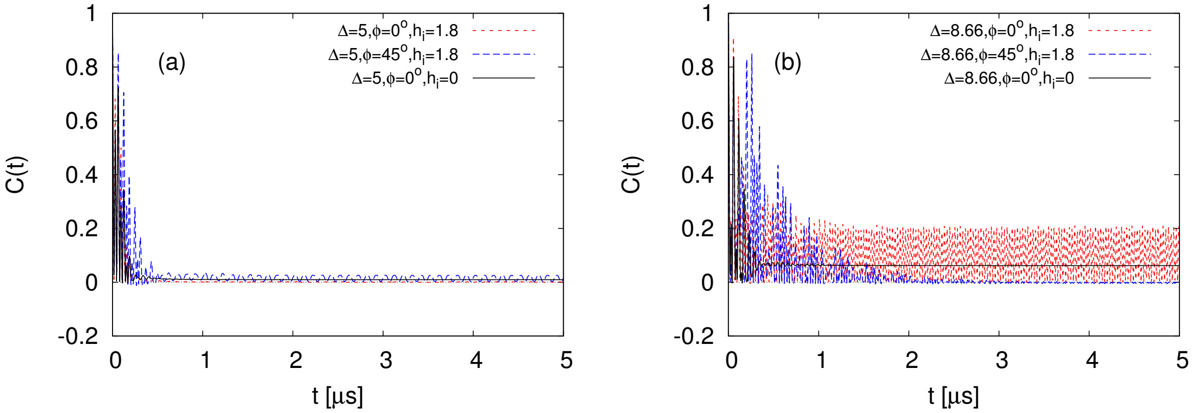


FIG. S15. (color online) Simulation results for the average of all spin-spin correlations (see Eq. (18)), for a system of $N_S = 28$ interacting spins (see Eq. (15)), spin-bath coupling $\lambda = 5$, $h_d = 15\,$MHz, and $h_i = 0.12 h_d = 1.8\,$MHz. a: $\Delta = 5\,$MHz, b: $\Delta = 8.66\,$MHz.

## X. FOURIER TRANSFORMS OF THE DATA PRESENTED IN FIG. 3 AND 6

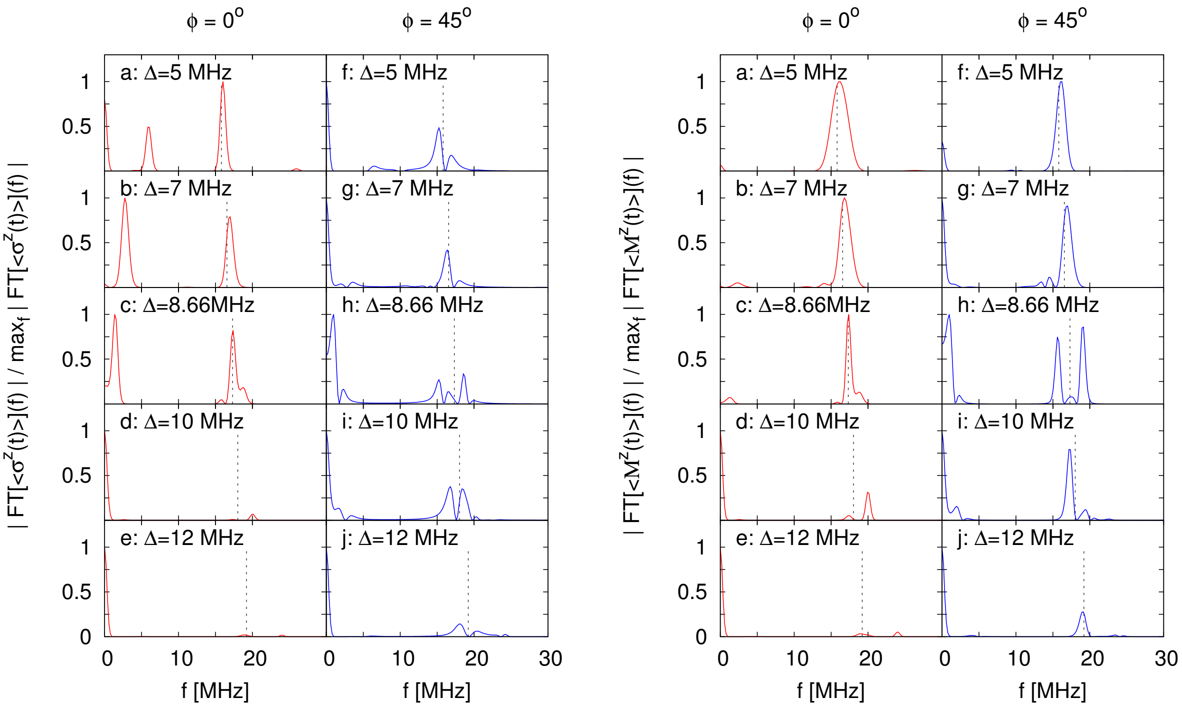


FIG. S16. (color online) Left: Fourier transforms of the data shown in Fig. 3, obtained by solving the TDSE for a spin interacting with a bath of $N_B = 28$ two-level systems. Right: Fourier transforms of the data shown in Fig. 7, obtained by solving the TDSE with Hamiltonian Eq. (15) for a system of $N_s = 28$ interacting spins.

## XI. FIGS. 1–3, AND 7 OF THE MAIN TEXT

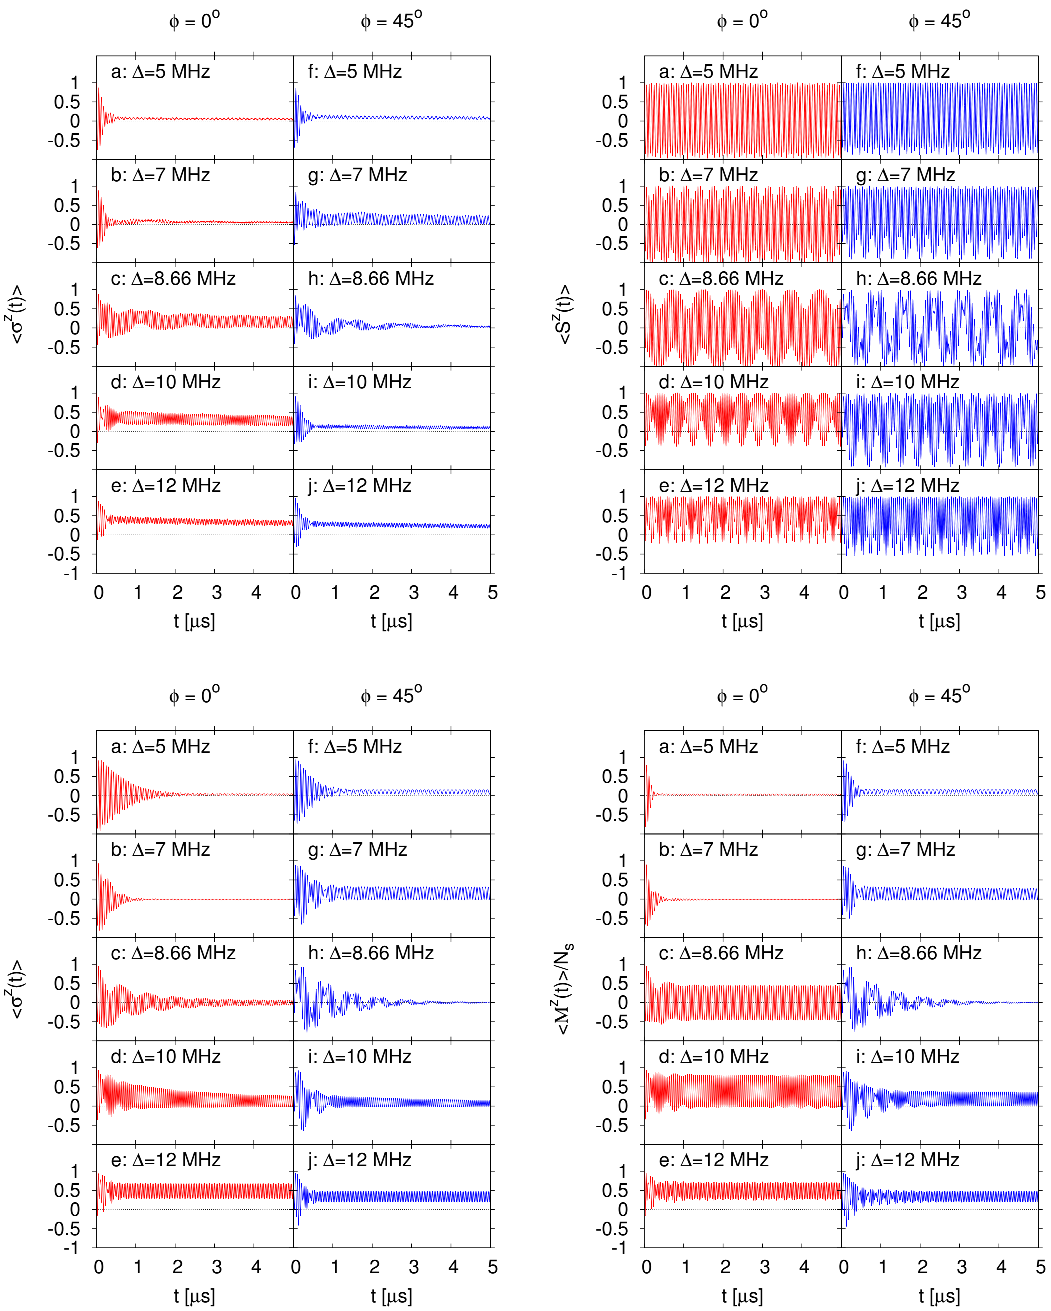


FIG. S17. (color online) Top left: Fig. 1 of the main text. Experimental data of the Rabi oscillations in $CaWO_4$:$Gd^{3+}$ at $T = 40\,\mathrm{K}$ for different values of the detuning $\Delta$, phase differences $\phi = 0°$ and $\phi = 45°$, (relative to an offset of $\approx 50°$ between the drive and image drive), and amplitudes $h_d = 15\,\mathrm{MHz}$ and $h_i = 0.12h_d = 1.8\,\mathrm{MHz}$, respectively. Top right: Fig. 2 of the main text. Simulation results obtained by solving the TDSE for the Hamiltonian Eq. (3), describing a single spin subject to the time-dependent magnetic field $\mathbf{B}(t) = 2\pi(h_d \sin\phi - h_i \sin(4\pi t\Delta + \phi), h_d \cos\phi + h_i \cos(4\pi t\Delta + \phi), \Delta)^{\mathrm{T}}$, with the amplitudes $h_d = 15\,\mathrm{MHz}$ and $h_i = 0.12h_d = 1.8\,\mathrm{MHz}$.For additional information, see sections I–II. Top left: Fig. 3 of the main text. Simulation results for the magnetization, as obtained by solving the TDSE for Hamiltonian Eq. (11), describing the single-spin system S coupled to a spin bath, both subject to a time-dependent magnetic field. The bath consists of $N_{\mathrm{B}} = 28$ interacting spins, the spin-bath coupling $\lambda = 6$, $J = 1\,\mathrm{MHz}$, $K = 10\,\mathrm{MHz}$, $h_d = 15\,\mathrm{MHz}$, and $h_i = 0.12h_d = 1.8\,\mathrm{MHz}$. Top right: Fig. 7 of the main text. Simulation results obtained by solving the TDSE with Hamiltonian Eq. (17) for a system of $N_{\mathrm{S}} = 28$ interacting spins, spin-bath coupling $\lambda = 5$ and microwave field inhomogeneity $\delta = 0.1$.

[S1] S. Bertaina, R. Vezin, H. De Raedt, and I.Chiorescu, Experimental protection of quantum coherence by using a phase-tunable image drive, Sci. Rep. , 10:21643 (2020).
[S2] J. Johansson, P. Nation, and F. Nori, QuTiP 2: A Python framework for the dynamics of open quantum systems, Comput. Phys. Commun. **184**, 1234 (2013).
[S3] H. De Raedt, B. Barbara, S. Miyashita, K. Michielsen, S. Bertaina, and S. Gambarelli, Quantum simulations and experiments on Rabi oscillations of spin qubits: Intrinsic vs extrinsic damping, Phys. Rev. B **85**, 014408 (2012).
[S4] H.-P. Breuer and F. Petruccione, *The Theory of Open Quantum Systems* (Oxford University Press, Oxford, 2002).
[S5] F. Jin, D. Willsch, M. Willsch, H. Lagemann, K. Michielsen, and H. De Raedt, Random state technology, J. Phys. Soc. Jpn. **90**, 012001 (2021).
